# Supplementary material for: SAFER: Safe Collision Avoidance using Focused and Efficient Trajectory Search with Reinforcement Learning
Source: arXiv:2209.11789 source file (2023-06-28)
Supplement: Supplementary file 1 [file appendix.tex]

\begin{appendices}
\begin{algorithm}[t!]
\caption{Training Algorithm}
\begin{algorithmic}[1]
\State Initialize experience buffer $\mathcal{D} \leftarrow \emptyset$
\State Randomly initialize RL network parameters $\theta$
\For{learning epochs}
    \State $(v_{\rm ref}, \omega_{\rm ref}) \leftarrow$ control command
    \State $s_t \leftarrow$ \{sensor scans, $v, w, v_{\rm ref}, \omega_{\rm ref}$\}
    \If{maximum braking required}
        \State $\sigma_t \leftarrow 1$, perform maximum braking 
        \State $a_t, (v_c, \omega_c) \leftarrow {\rm Null}, (-v_{\rm max}, 0)$
    \Else
        \State $\sigma_t \leftarrow 0$, do not perform maximum braking 
        \If{collision avoidance required}
            \State $a_t \leftarrow [throttle, turn] \leftarrow$ RL policy network
            \State $(v_c, \omega_c) \leftarrow$ targeted search with $\{s_{t}, a_{t}\}$
        \Else
            \State $a_t, (v_c, \omega_c) \leftarrow {\rm Null}, (v_{\rm ref}, \omega_{\rm ref})$
        \EndIf
    \EndIf
    \If{$a_{t-1}$ not ${\rm Null}$}
        \State $r_{t-1}\leftarrow$ eq.~\eqref{eq:reward} with $\{s_{t-1}, a_{t-1}, \sigma_t\}$
        \State $\mathcal{D} \leftarrow \{s_{t-1}, a_{t-1}, r_{t-1}, \sigma_t\}$
    \EndIf
    \State command robot with $(v_c, \omega_c)$
\State use $\mathcal{D}$ to update $\theta$ using RL
\EndFor
\end{algorithmic}
\label{procedure:LAMB}
\end{algorithm}

\section{Tuning Collision Avoidance Hyperparameters}
In order to aid the reader in understanding how to tune the more important collision avoidance parameters in our work, $[\beta, n_v, n_\omega, \gamma, \delta]$, we provide a brief discussion. 
\begin{itemize}
    \item $\beta>1$ controls the planning look-ahead multiplier. Larger settings causes the RL-guided search to be triggered more often for collision avoidance, which can be desirable to a certain extent; too large of a setting can negatively affect the human control experience due to being overly conservative. We recommend tuning this parameter based on the desired level of collision avoidance interruption to user control. We set $\beta=2$.
    \item $n_v, n_\omega$ determine how many linear and angular velocities are sampled from the dynamic window, resulting in $n_v n_\omega$ samples. We maximize the values of $n_v, n_\omega$ up to the point where the standard DWA search achieves a planning cycle latency of the desired $t_r$ (100ms in our setting). Depending on the robotic platform, one can increase the value of $n_v$ compared to $n_\omega$ or vice-versa if the window size is larger in either direction. 
    \item $\gamma, \delta \in (0, 1)$ control the size of the targeted RL search. $\delta$ should be set such that the search time $t_{search}$ resulting from the number of samples $\delta^2 n_v n_\omega$ offsets the inference time of the RL policy $t_{\pi}$; $t_{search} \leq t_r - t_{\pi}$. $\gamma$ is then set to achieve the desired search granularity compared to the standard DWA search $\gamma / \delta$, ideally $\gamma / \delta \leq 1$ (more granular). 
\end{itemize}
\end{appendices}
